# Supplementary material for: Anomalous Diffusion along Metal/Ceramic Interfaces
Source: arXiv:1807.04708 source file (2018-07-12)
Supplement: Supplementary file 1 [file SI_Anomalous_Diffusion_final.pdf]

# Supplementary Information (SI)

# Anomalous Diffusion along Metal/Ceramic Interfaces

Aakash Kumar[†,1,*] Hagit Barda,[2,*] Leonid Klinger,[2] Michael W. Finnis,[3,4] Vincenzo Lordi,[5] Eugen Rabkin,[2] and David J. Srolovitz[1,6,†]

[1] *Department of Materials Science and Engineering, University of Pennsylvania, Philadelphia PA 19104, USA*

[2] *Department of Materials Science and Engineering, Technion - Israel Institute of Technology, 3200003 Haifa, Israel*

[3] *Department of Materials and Department of Physics, Imperial College, London SW7 2AZ, UK*

[4] *Thomas Young Center, London SW7 2AZ, UK*

[5] *Materials Science Division, Lawrence Livermore National Laboratory, Livermore, CA 94550, USA*

[6] *Department of Mechanical Engineering and Applied Mechanics, University of Pennsylvania, Philadelphia, PA 19104, USA*

[*] These authors contributed equally to this work.

[†] corresponding authors: aakashk@seas.upenn.edu, srol@seas.upenn.edu

## I. GROOVING MODEL FOR CIRCULAR GRAINS

Our model describes the evolution of the surface topography of a thin metal film deposited on a ceramic substrate via simultaneous surface, grain boundary (GB), and interface self-diffusion of the film material (diffusion within the metal film grains and in the substrate are assumed to be zero). The analyzed system (Fig. 2.a, manuscript) consists of a cylindrical metal grain of constant radius $R_0$ embedded in a continuous metal film. We explicitly assume that at the outer (circular) edge of the continuous metal film (i.e., at $R_{out}$) both surface and interface diffusion fluxes vanish. This radius may be thought of as half the distance between neighboring sinking grains. The substrate is assumed to be immobile during annealing. Table I introduces all of the symbols used in the model.

TABLE I. List of symbols used.

| Symbol | Description |
|---|---|
| $R_0$ | radius of the cylindrical sinking grain |
| $R_{out}$ | radius of the outer grain; diffusion fluxes vanish here |
| $j_{s(r)}$ | surface flux |
| $\mu_{s(r)}$ | chemical potential at the surface |
| $D_s$ | surface diffusion coefficient |
| $\nu_s$ | number of mobile atoms per unit surface area |
| $\nu_{gb}$ | number of mobile atoms per unit GB area |
| $\nu_i$ | number of mobile atoms per unit interface area |
| $k$ | Boltzmann constant |
| $T$ | temperature in Kelvin |
| $u$ | velocity of the crystal lattice drift normal to the substrate |
| $\gamma_{gb}$ | GB energy (per unit area) |
| $j_{gb}$ | GB diffusion flux |
| $D_{gb}$ | GB diffusion coefficient |
| $D_i$ | Interface diffusion coefficient |
| $\mu_s^{gb}$ | chemical potential at the groove root (point A) |
| $\mu_i^{gb}$ | chemical potential at the intersection of the GB and the interface (point B) |
| $h$ | distance between the grain boundary root (point A) and the interface |
| $\mu_i$ | chemical potential at the interface |
| $\Omega$ | atomic volume |

### A. Surface diffusion

The driving force for surface diffusion is the curvature of the surface (i.e., capillarity; the Gibbs-Thomson effect). Therefore, the surface flux and the chemical potential at the surface

are given by:

$$j_s(r) = -\frac{D_s\nu_s}{kT}\frac{\partial\mu_s}{\partial\mu r} \tag{1}$$

$$\mu_{s(r)} = \Omega\gamma_s\frac{\partial}{r\partial r}\left(r\frac{\partial y}{\partial r}\right). \tag{2}$$

The evolution of the film surface profile $y(r,t)$ with respect to the immobile substrate is described by:

$$\frac{\partial y}{\partial t} = -\Omega\frac{\partial}{r\partial r}\left(rj_s\right) + u, \tag{3}$$

where $u$ is the lattice drift due to the accretion of atoms at the metal/ceramic interface.

We employ the following boundary conditions for (1) and (3):

$$\left.\frac{\partial y}{\partial r}\right|_{r=0} = \left.\frac{\partial y}{\partial r}\right|_{r=R_{out}} = 0; \qquad j_s|_{r=0} = j_s|_{r=R_{out}} = 0 \tag{4}$$

$$\left.\frac{\partial y}{\partial r}\right|_{r=R_0+} - \left.\frac{\partial y}{\partial r}\right|_{r=R_0-} = \gamma_{gb}/\gamma_s; \qquad j_s|_{r=R_0+} - j_s|_{r=R_0-} = -j_{gb}. \tag{5}$$

The boundary conditions in (4) follow from the symmetry of the system and the definition of $R_{out}$. The boundary conditions in (5) results from the equilibrium and mass balance conditions at the root of GB groove (point A).

### B. Grain boundary diffusion

We assume that the material diffusing along the grain boundary does not accumulate there (otherwise, large bi-axial stresses in the film; these would shutdown any mass accumulation along the GB [1]). The atoms diffusing along the grain boundary arrive at the film-substrate interface and may diffuse along the interface. Any atom accumulation along the interface will cause an upward drift of the crystal lattice of the film and concomitant change of the surface profile (note that, unlike at the GB, atom accumulation at the interface may occur because the surface is traction free). The rate of this upward drift is obtained from the mass conservation condition:

$$u = j_{gb}\,\frac{2\pi R_0}{\pi R_{out}^2}, \tag{6}$$

where $j_{gb}$ is the constant grain boundary flux

$$j_{gb} = \frac{D_{gb}\nu_{gb}}{kT}\,\frac{\mu_s^{gb} - \mu_i^{gb}}{h}. \tag{7}$$

It should be noted that the continuity of chemical potential implies that it is the same on all sides of the groove root, which means $\mu_s^{gb} \equiv \mu_s(R_0^+) = \mu_s(R_0^-)$.

### C. Interface diffusion

The diffusion flux along the metal/ceramic interface, $j_i$, is given by

$$j_i(r) = -\frac{D_i\nu_i}{kT}\,\frac{\partial\mu_i}{\partial r}. \tag{8}$$

The material accumulation at the interface should be uniform (otherwise, large bending stresses would develop in the film, leading to a large strain energy); this implies that the interface diffusion flux divergence is constant:

$$\frac{1}{r}\frac{\partial(rj_i)}{\partial r} = const. \tag{9}$$

Employing arguments similar to those used in formulation of boundary conditions (4)-(5) yields the following set of boundary conditions for diffusion along the interface (9):

$$j_i(R_{out}) = j_i(0) = 0; \qquad\qquad j_i(R_0+) - j_i(R_0-) = j_{gb}. \tag{10}$$

Combining (9) and (10) yields the following expression for the interface diffusion flux:

$$j_i(r) = -j_{gb}\,\frac{R_0}{R_{out}^2}\begin{cases} r & 0 < r < R_0 \\ r - \frac{R_{out}^2}{r} & R_0 < r < R_{out}. \end{cases} \tag{11}$$

Combining (8) and (11) and the condition of chemical potential continuity $\left(\mu_i^{gb} \equiv \mu_i(R_0+) = \mu_i(R_0-)\right)$ results in the following expression for the interface chemical potential:

$$\frac{D_i \nu_i}{kT}\,\mu_i(r) = \frac{D_i \nu_i}{kT}\,\mu_i^{gb} - j_{gb}\,\frac{R_0}{R_{out}^2} \begin{cases} 0.5(R_0^2 - r^2) & 0 < r < R_0 \\ 0.5(R_0^2 - r^2) + R_{out}^2 \ln{(r/R_0)} & R_0 < r < R_{out}. \end{cases} \tag{12}$$

### D. Connection between grain boundary and interface diffusion

The average value of the interface chemical potential can be determined using a thought experiment in which an infinitesimally thin disc of film material is inserted at the interface. The total energy of the system would then increase due to the formation of a new grain boundary segment around the cylindrical grain. If this increase is exactly compensated by the energy change due to the influx of interface atoms [2, 3], we find:

$$\int_0^{R_{out}} 2\pi r \mu_i(r) dr = 2\pi R_0 \gamma_{gb} \Omega. \tag{13}$$

Combining (7),(12) and (13) gives an expression for the GB diffusion flux as a function of the material parameters $(D_{gb}, \nu_{gb}, D_i, \nu_i, \gamma_{gb})$, the geometry of the system $(h, R_0, R_{out})$, and only one chemical potential (linking the surface and interface diffusion, $\mu_s^{gb}$):

$$j_{gb} = \frac{D_{gb}\nu_{gb}D_i\nu_i\left[\mu_s^{gb} - 2R_0\gamma_{gb}\Omega/R_{out}^2\right]}{kT\left[hD_i\nu_i + R_0 D_{gb}\nu_{gb}\; f(\frac{R_0}{R_{out}})\right]}, \tag{14}$$

where $f(x) = x^2 - 3/4 - \ln x$. Combining (1), (2), (6) and (14) yields a second order differential equation (3), the solution of which is $y(r,t)$.

In Fig. 2b of the manuscript, the calculated $y(r,t)$ profiles for three different values of interface diffusivities are plotted at a time corresponding to when the GB groove root arrives at the interface. This corresponds to hole nucleation and the onset of solid state dewetting. The values of the grain boundary and surface self-diffusivities (defined as the product of the diffusion coefficient, the number of mobile atoms per unit area, and the atomic volume) employed in simulations were $1.2\times10^{-21}\text{m}^3/\text{s}$ and $10^{-21}\text{m}^3/\text{s}$ respectively [4, 5]. The surface and grain boundary energies of Ni were taken to be 2.1 $\text{J/m}^2$ and 1 $\text{J/m}^2$, respectively [6, 7]. The inner and outer grain diameters were set to $R_0 = 0.25\ \mu$m and $R_{out} = 3\ \mu$m, respectively.

The three profiles in Fig. 2b of the manuscript correspond to three value of the interface diffusivity, $D_i = 0$, $D_i = D_{gb}$ and $D_i = 5D_{gb}$, at the times that the GB groove hits the substrate, i.e., 814 s, 480 s, and 232 s, respectively. One can see that increasing the interface diffusivity shortens the time needed for nucleation of a hole. Also, the amplitude of the hole rim elevation decreases with increasing interface diffusivity, creating an illusion of the 'mass deficit'. It should be also noted that due to the axisymmetric geometry of the problem the upward drift of the film is very small and hardly discernable in this figure. In addition, Fig. 1 presents profiles of $y(r,t)$ for two different values of interface diffusivity and the same annealing time, showing the contribution of the interface diffusion to the acceleration of the central grain sinking rate.

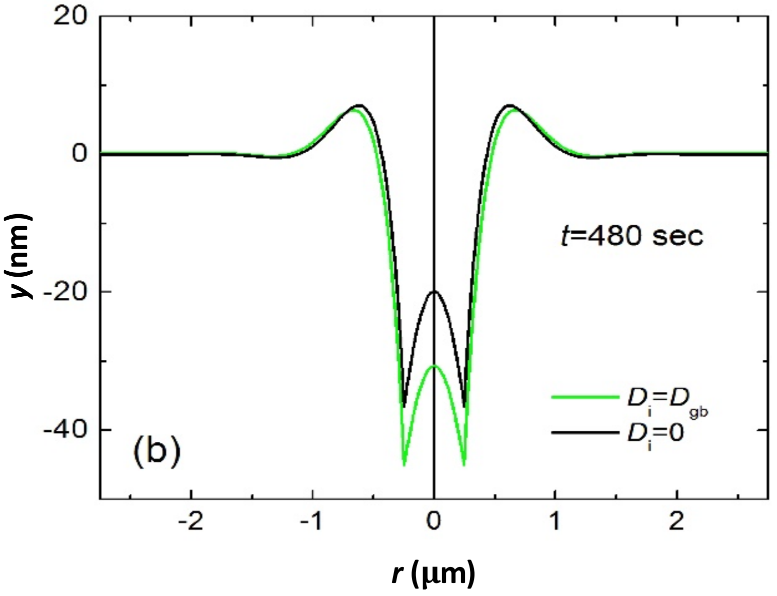


FIG. 1. Surface topography profiles *y(r)* with and without interface diffusivity for the same time duration, demonstrating that the grain has sunk faster at a greater acceleration due to interface diffusion.

In our experiments, we determined the volume of Ni accumulated in the ridge surrounding the hole, and the volume of Ni rejected by the hole, with respect to the average height of the unperturbed thin film surface far from the hole. To mimic this experimental procedure, we performed a similar mass balance analysis employing the simulated profiles $y(r,t)$, and using $y\,(r = R_{out}, t)$ as a reference zero point. The resulting dependence of the volume imbalance $\Delta V$ on annealing time is shown in Fig. 2c(main text). The apparent mass imbalance

increases with increasing interface diffusivity. The simulations reproduce the experimentally determined mass imbalance ($5 \times 10^{-3} \mu m^3$ of Ni after 10 min annealing) for $D_i \approx D_{gb}$. Thus, the self-diffusion coefficient of Ni along the Ni-sapphire interface at 700°C is of the same order of magnitude as the self-diffusion coefficient along a random large angle grain boundary in Ni.

## II. First-principles calculations

### A. FCC Ni

The lattice properties of face centered cubic (FCC) Ni, as predicted by SCAN, are shown in Table II along with the PBE and experimental data. Readers are referred to an exhaustive comparison in the literature [8] for additional data on SCAN.

TABLE II. Lattice constant $a_0$ and surface energy $\gamma_{(111)}$ of FCC Ni.

| Property | Expt. | SCAN (this work) | PBE(GGA) (this work) |
|---|---|---|---|
| $a_0$ (Å) | 3.52 [9] | 3.45 | 3.52 |
| $\gamma_{(111)}$ (J/m$^2$) | 2.24 [10] | 2.18 | 1.92 |

### B. Sapphire

$\alpha$-$Al_2O_3$ (sapphire) crystallizes in a trigonal structure with the space group R$\bar{3}$C, number 167 - see Fig. 2. The lattice parameters and formation enthalpy of sapphire calculated with the meta-GGA functional SCAN show much better agreement with the experimental results than GGA as shown in Table III below.

TABLE III. Lattice properties of $\alpha$-$Al_2O_3$.

| Property | PBE(GGA) (*this work) | Experiment | SCAN (this work) |
|---|---|---|---|
| a (Å) | 4.81 [11], 4.81* | 4.76 [12] | 4.75 |
| c (Å) | 13.14 [11], 13.12* | 12.99 [12] | 12.96 |
| $\Delta H_f$ (eV) | -16.71 [13], -15.5* | -17.37 [14] | -17.5 |
| $\gamma_{(0001)}$ (J/m$^2$) | 1.59 [15], 1.54* | 2.60 [16] | 1.98 |
| $E_g$ (eV) | 5.85 [11], 5.81* | 8.80 [17] | 7.18 |

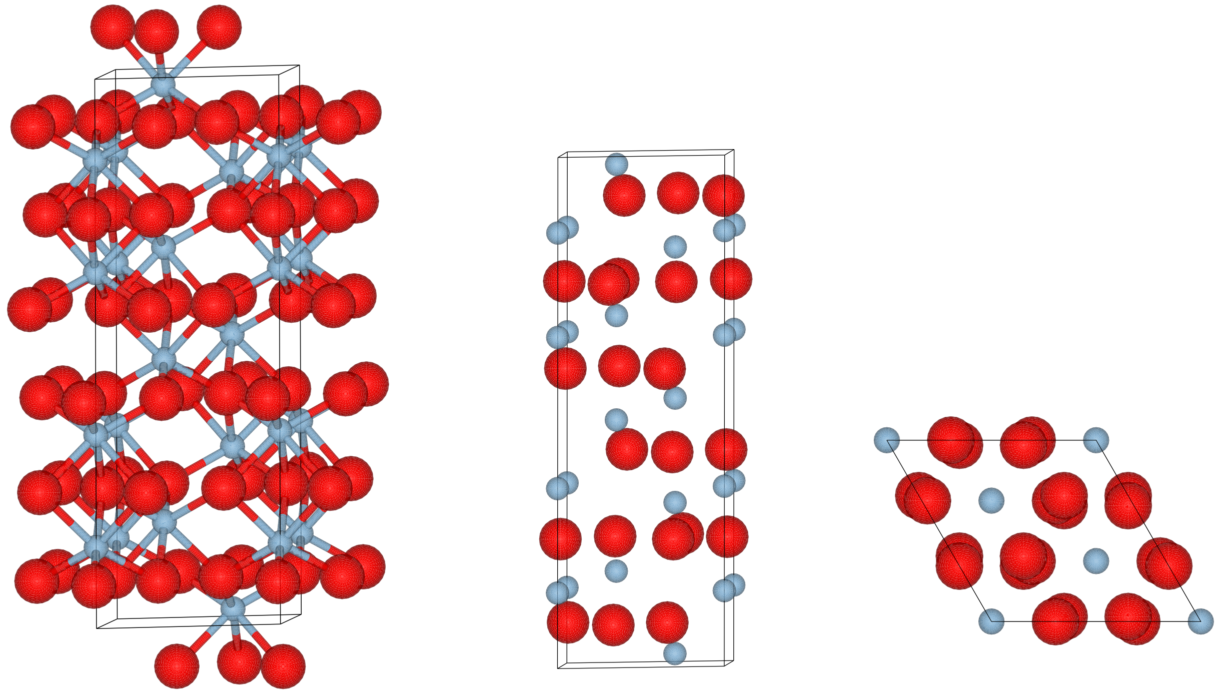

(a) 3D view (b) side-view (c) top-view

FIG. 2. Three views of the $\alpha$-$Al_2O_3$ crystal, showing the location of the O (red) and Al (blue) atoms.

### C. Vacancies in Sapphire

The formation energy of a vacancy of charge $q$ in a solid $\mathrm{V}_X^q$ can be calculated using [18]

$$E_{\mathrm{f}}^{\mathrm{V}_{\mathrm{X}}^{q}(\infty)} = E_{\mathrm{defect}} - E_{\mathrm{perfect}} - \Sigma n_i \mu_i + qE_F + \Delta q, \tag{15}$$

where $E_{\mathrm{f}}^{\mathrm{V}_{\mathrm{X}}^{q}}(\infty)$ is the bulk formation energy of the vacancy in charge state $q$, $E_{\mathrm{defect}}$ and $E_{\mathrm{perfect}}$ are the computed energies of the supercell with and without the defect respectively where the total volume has been fixed at the value appropriate for the perfect crystal, $n_i$ is the number of atoms removed ($n_i < 0$) from the system to create the vacancy, $\mu_i$ is the chemical potential of the species being removed, $E_F$ is the Fermi energy and $\Delta q$ is a correction related to the finite size of the supercell [19]. For our calculations, we chose a 120 atom sapphire supercell that is a 2x2x1 replication of the 30 atom unit cell of $\alpha$-$Al_2O_3$ shown in Fig. 2.

In the above equation, the chemical potential of species $i$ is $\mu_i = \mu_{\mathrm{i}}^0 + \Delta\mu_i$. We determine

the bounds on the chemical potentials for Al and O as below:

$$\mu_{\mathrm{Al}} \leq \mu^0_{\mathrm{Al}}, \quad \mu_{\mathrm{O}} \leq \mu^0_{\mathrm{O}} \tag{16}$$

$$2\Delta\mu_{\mathrm{Al}} + 3\Delta\mu_{\mathrm{O}} = \Delta H_{f\,\mathrm{Al_2O_3}}. \tag{17}$$

These bounds ensure that Ni is not oxidized nor sapphire reduced. Equation (17) implies that we need know only the the O or Al chemical potentials, but not both; here, we focus on the oxygen chemical potential since it is easier to manipulate experimentally (via the oxygen partial pressure).

Together, Eqs. (16) and (17) set the lower and upper bounds on the oxygen partial pressures ($p^{\mathrm{min}}_{\mathrm{O_2}}$ and $p^{\mathrm{max}}_{\mathrm{O_2}}$) to ensure that the Ni/$Al_2O_3$ is stable. This implies that the Al chemical potential, $\mu_{\mathrm{Al}} = \mu^0_{\mathrm{Al}}$:

$$\mu_{\mathrm{O}} = \mu^0_{\mathrm{O}} + \frac{1}{3}\Delta H_{f\,\mathrm{Al_2O_3}}. \tag{18}$$

The $p^{\mathrm{max}}_{\mathrm{O_2}}$ conditions represent the upper bound on the O chemical potential; we choose this as the limit above which Ni is oxidized to form NiO. Hence, we can write,

$$\Delta\mu_{\mathrm{Ni}} + \Delta\mu_{\mathrm{O}} = \Delta H_{f\,\mathrm{NiO}}. \tag{19}$$

Combining Eq. (19) with $\mu_{\mathrm{Ni}} = \mu^0_{\mathrm{Ni}}$, we get

$$\mu_{\mathrm{O}} = \mu^0_{\mathrm{O}} + \Delta H_{f\,\mathrm{NiO}} \tag{20}$$

and $\mu_{\mathrm{Al}}$ can be obtained from (18). These $p^{\mathrm{min}}_{\mathrm{O_2}}$ and $p^{\mathrm{max}}_{\mathrm{O_2}}$ limits of $\mu_{\mathrm{O}}$ are shown in Table IV. $p^{\mathrm{max}}_{\mathrm{O_2}}$ favor the interface formed by O-terminated sapphire while the $p^{\mathrm{min}}_{\mathrm{O_2}}$ conditions lead to the interface formed by 2Al-terminated sapphire.

TABLE IV. Values of the chemical potentials of O, Al and Ni for O-poor ($p^{\mathrm{min}}_{\mathrm{O_2}}$) and O-rich ($p^{\mathrm{max}}_{\mathrm{O_2}}$) conditions.

| Conditions | $\mu_{\mathrm{O}}$ | $\mu_{\mathrm{Al}}$ | $\mu_{\mathrm{Ni}}$ |
|---|---|---|---|
| $p^{\mathrm{min}}_{\mathrm{O_2}}$ | -11.86 | -7.75 | -16.07 |
| $p^{\mathrm{max}}_{\mathrm{O_2}}$ | -7.60 | -14.13 | -16.07 |

The Fermi energy plays an important role when the vacancy is charged - see Eq. (15). For the range of point defect energies in sapphire, the Fermi energy may vary from the valence band maximum (VBM) to the conduction band minimum (CBM) or

$$0 \leq E_F \leq 7.18\,\mathrm{eV}. \tag{21}$$

By varying the Fermi energy (electron chemical potential), we can compare the formation energy of defects in different charge states and also locate the points of transitions from one charge state to another.

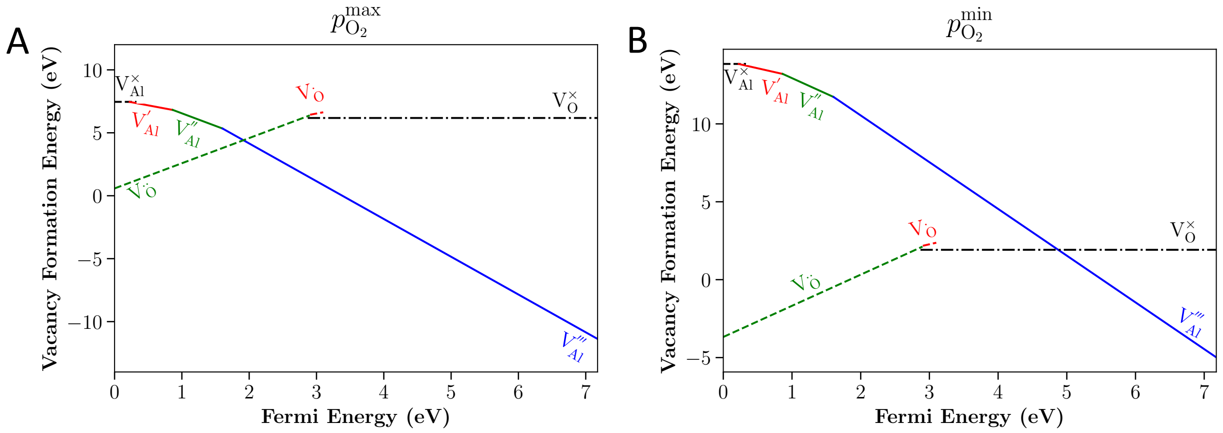


FIG. 3. Al and O vacancy formation energies for (*A*) $p_{\mathrm{O}_2}^{\max}$ and (*B*) $p_{\mathrm{O}_2}^{\min}$ conditions.

We calculate the Al (charge states 0, -1, -2 and -3, represented in Kröger-Vink notation as $\mathrm{V}_{\mathrm{Al}}^{\times}$, $\mathrm{V}_{\mathrm{Al}}^{'}$ , $\mathrm{V}_{\mathrm{Al}}^{''}$, and $\mathrm{V}_{\mathrm{Al}}^{'''}$) and O vacancy (charge states 0, +1 and +2, i.e., $\mathrm{V}_{\mathrm{O}}^{\times}$, $\mathrm{V}_{\dot{\mathrm{O}}}$, and $\mathrm{V}_{\ddot{\mathrm{O}}}$) in the 120 atom sapphire supercell. As previously discussed, the chemical potential of O can be varied between the two extremes, $p_{\mathrm{O}_2}^{\min}$ (O-poor) and $p_{\mathrm{O}_2}^{\max}$ (O-rich). Figure 3 shows the formation energy of vacancies in pure sapphire under these conditions. The stable point vacancies are $\mathrm{V}_{\mathrm{O}}^{\times}$ and $\mathrm{V}_{\mathrm{Al}}^{'''}$ near the mid-point of the band gap and $\mathrm{V}_{\ddot{\mathrm{O}}}$ and $\mathrm{V}_{\mathrm{Al}}^{\times}$ near the balence band edge. $\mathrm{V}_{\dot{\mathrm{O}}}$ is never stable - consistent with earlier caclulations [20]. Since we focus on vacancies in sapphire near the Ni/sapphire interface, we only consider neutral vacancies (as discussed in the manuscript).

Returning to the M1 interface (Fig. 4c of the main text), we note that while the Al vacancy formation energy $E_{\mathrm{f}}^{\mathrm{V}_{\mathrm{Al}}^{\times}}$ in 2Al-terminated sapphire case is relatively small near the interface, but does not appear to approach its bulk value $E_{\mathrm{f}}^{\mathrm{V}_{\mathrm{Al}}^{\times}}(\infty, p_{\mathrm{O}_2}^{\min})$ far into the sapphire.

Examination of the atomic structure of this vacancy shows that it is different from that observed in bulk sapphire [21], even at the maximum separation from the interface in our computational cell ($\sim 6$Å). For the same interface, the O vacancy formation energy drops from 1.86 eV in the bulk to 1.34 eV near the interface at $p_{O_2}^{\min}$.

### D. Lateral translations at the Ni/sapphire interface

The Ni terminations can be either A, B or C according to the classical description of the stacking of FCC {111} planes. These terminating Ni layers represent different translations of the Ni crystal parallel to the interface. We explore this configuration space by considering these three cases for each sapphire termination, leading to 9 total interfacial structures. These Ni lattice shifts for O-terminated sapphire are shown in Fig. 4.

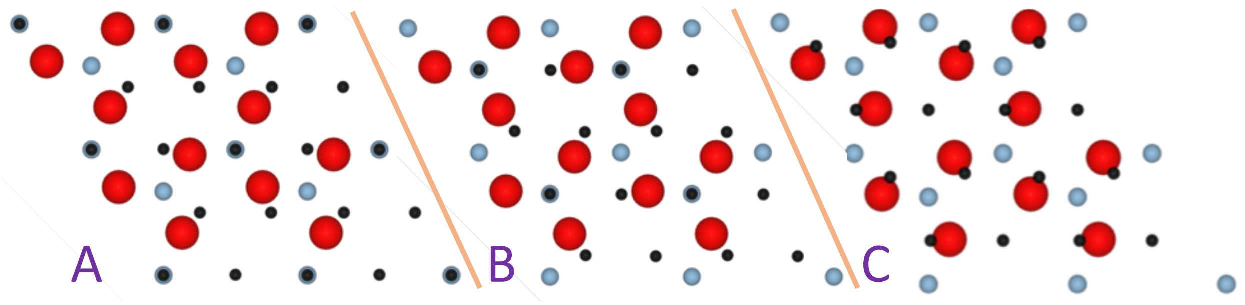


FIG. 4. Top view of the M1 Ni(111)$[1\bar{1}0] \| \alpha$-$Al_2O_3(0001)[11\bar{2}0]$ (O-terminated) with the the terminating Ni {111} plane A, B or C. Ni, Al and O are indicated by black, blue and red.

### E. Interface Energy

The $\alpha$-$Al_2O_3$ (0001) free surface has received extensive attention in the literature and the Al-terminated stoichiometric free surface was determined to be most stable over the entire range of oxygen chemical potentials for which $\alpha$-$Al_2O_3$ is stable. However, at the Ni(111)/$\alpha$-$Al_2O_3$(0001) interface, the $Al_2O_3$ may have different terminations depending on the oxygen chemical potential. The Ni/sapphire (0001) interface energy $\gamma_i$ for different interface terminations may be used to determine the stable interface structures at different chemical potentials, as discussed in the main text. The interface energy can be calculated as,

$$\gamma_{\rm i} = \frac{(G_0 - N_O\mu_{\rm O} - N_{\rm Al}\mu_{\rm Al} - N_{\rm Ni}\mu_{\rm Ni})}{A}, \tag{22}$$

where A is the interface area, $N_{\rm O}$, $N_{\rm Al}$, $N_{\rm Ni}$ are the number of O, Al and Ni atoms in the system and, $\mu_{\rm O}$, $\mu_{\rm Al}$ and $\mu_{\rm Ni}$ are the chemical potentials of O, Al and Ni. $G_0$ is the total energy of the interface from the DFT calculations. Using the constraint 2 $\mu_{\rm Al}+3\mu_{\rm O} = \mu_{\rm Al_2O_3}$, we can rewrite Eq. (22) as Eq. (23).

$$\gamma_{\rm i} = \frac{(G_0 - \frac{1}{2}N_{\rm Al}\mu^0_{\rm Al_2O_3} - [N_{\rm O} - \frac{3}{2}N_{\rm Al}]\mu_{\rm O} - N_{\rm Ni}\mu_{\rm Ni})}{A} \tag{23}$$

Equations (16), (17) and (19) define the range of oxygen chemical potentials ($\mu_{\rm O}$) of interest. The interface energies for all the interfaces formed by the three sapphire(0001) and the three Ni terminations are shown in Fig. 3b of the main text. Both the 2Al-terminated and O-terminated sapphire interfaces have a large stability region (see main text).

## F. Vacancy Migration Energy in FCC Ni and Ni/sapphire Interface

Table V shows the Ni migration energies calculated using nudged elastic band calculations in bulk Ni and near the Ni/sapphire interface as obtained using the SCAN functional (see the main text). To determine accurate migration energies in FCC Ni and along the Ni/sapphire interface, we use a supercell twice the size of that used for the Ni and M1 interface energy calculations, in $b$ direction. The vacancy migration energy for perfect crystal Ni, obtained using SCAN for our hexagonal supercell, are in reasonable agreement with those obtained using PBE-GGA (i.e., 1.08 eV) [22] for a relaxed (3x3x3)$a_0$ cubic supercell as shown in Table V.

TABLE V. Vacancy migration energies in bulk Ni and two (111) Ni planes from the Ni/sapphire interface and at a coherent twin boundary and a large angle GB (LAGB) in NI.

| Position of the vacancy | Vacancy migration Energy ($E_{\rm m}^{\rm V_{Ni}^{\times}}$) | |
|---|---|---|
| | unstrained | strained(M1-epitaxy) |
| bulk | 1.08 [22], 1.06 | 1.00 |
| Coherent Twin ($\Sigma$ =3) | 0.99 [22] | – |
| LAGB ($\Sigma$ =9) | 0.35 [22] | – |
| Ni/sapphire Interface | – | 0.49 |

Figure 5 shows several images along the Ni vacancy migration path along the interface and the corresponding migration barrier is shown in Fig. 6.

The main result in Table IV is the comparison between the Ni migration energy in bulk

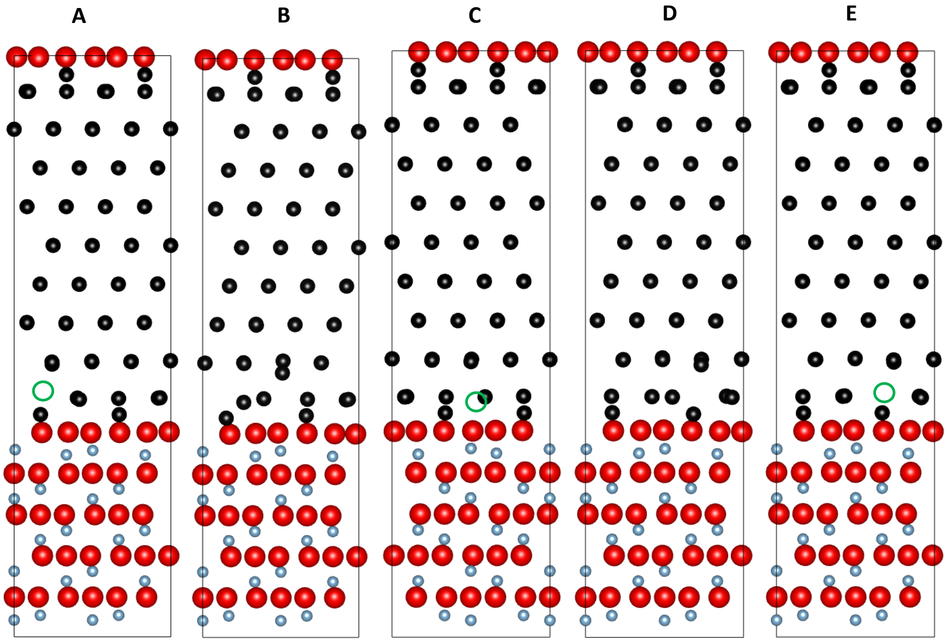


FIG. 5. Migration path of a Ni vacancy (green circle) along the interface.

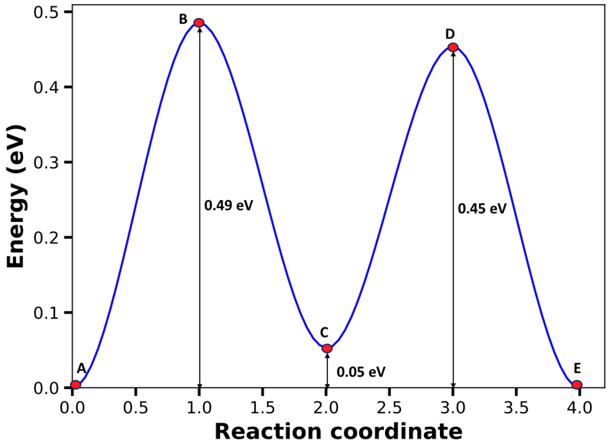


FIG. 6. The energy of a Ni vacancy along its migration path for diffusion along the Ni/sapphire interface. The points indicated by the letters and the vertical lines correspond to the subfigures in Fig. 5. The migration barrier is 0.49 eV (the greater of the two barriers).

Ni to that parallel to the interface (i.e., two (111) Ni planes from the Ni/sapphire interface) $E_{\rm m}^{\rm V_{Ni}^{\times}}(0, p_{O_2}^{\rm max})$. The vacancy migration energy near the interface is 0.49 eV; i.e., which is 49% that in bulk Ni (i.e., 1.00 eV). As discussed in the main text, an Al vacancy close to the interface on the sapphire side of the interface migrates to the Ni side of the interface giving rise to a Ni vacancy (Ni side) and a Ni interstitial on the sapphire side. This observation shown in Fig. 7 further suggests that the concentration of Ni vacancies at the interface is

very high.

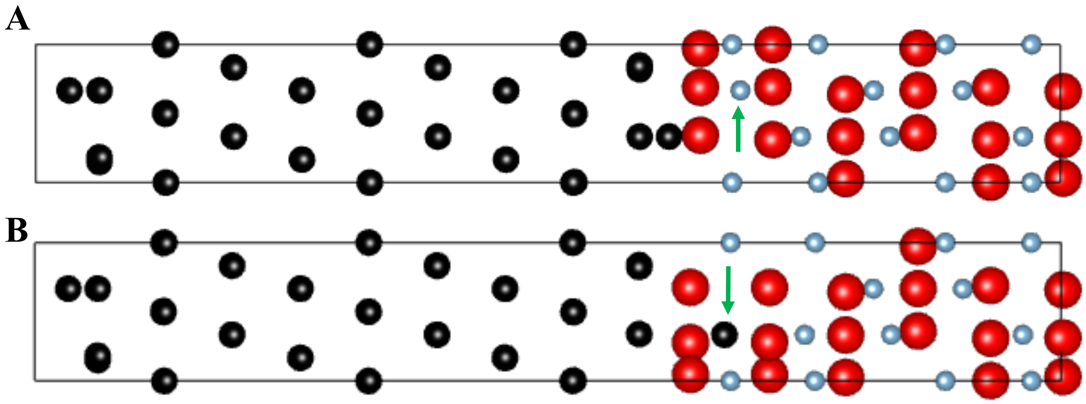


FIG. 7. Relaxation of the interface containing an Al vacancy. a) An Al atom (indicated by the arrow) is removed to form a Al vacancy. b) Relaxation of this interface with an Al vacancy shows that a Ni atom moves across the interface leaving behind a Ni vacancy and creating a Ni interstitial in the sapphire (indicated by the arrow).

## III. VACANCY FORMATION ENERGY: A GENERALIZED BOND BREAKING MODEL

We develop a simple, heuristic, bond breaking model to describe the vacancy formation energy at metal/ceramic interfaces. To form a vacancy within a metal requires breaking $N_b$ metal-metal bonds, $E_{\mathrm{f}}^{\mathrm{V}_{\mathrm{m}}^{\times}}(\infty) = N_b e_{\mathrm{mm}}$, where $e_{\mathrm{mm}}$ is a metal-metal (mm) bond energy. (NB: the effective number of bonds broken depends on the nature of bonding; for covalent bonds it proportional to the number of nearest neighbors $z$, whilst in metals, where bonding is more delocalized, it is more complicated, e.g., see [23].) The metal surface energy $\gamma_{\mathrm{m}}$ in such a model is the energy to break $N_s$ metal-metal (mm) bonds per unit area $\gamma_{\mathrm{m}} = N_s e_{\mathrm{mm}} \rho$, where $\rho$ is the planar density of atoms on the surface. Hence, $E_{\mathrm{f}}^{\mathrm{V}_{\mathrm{m}}^{\times}}(\infty) \approx (N_b/N_s)\gamma_{\mathrm{m}}/\rho$. The metal-ceramic (mc) interface energy is $\gamma_{\mathrm{i}} = \gamma_{\mathrm{m}} + \gamma_{\mathrm{c}} - N_i e_{\mathrm{mc}} \rho$, where $\gamma_{\mathrm{c}}$ is the surface energy of the ceramic, $N_i$ is the number of mc bonds, and $e_{\mathrm{mc}}$ is the metal-ceramic bond energy. The metal-ceramic work of adhesion is $W_{\mathrm{ad}} = \gamma_{\mathrm{m}} + \gamma_{\mathrm{c}} - \gamma_{\mathrm{i}} = N_i e_{\mathrm{mc}} \rho$. Hence the metal vacancy formation energy on the metal side of the mc interface implies breaking $N_i$ mc and $(N_b - N_s)$ mm bonds: $E_{\mathrm{f}}^{\mathrm{V}_{\mathrm{m}}^{\times}}(0) = N_i e_{\mathrm{mc}} + (N_b - N_s) e_{\mathrm{mm}} = [(N_b - N_s)\gamma_{\mathrm{m}} + N_s W_{\mathrm{ad}}]/N_s \rho$. The ratio of the metal vacancy formation energy at the metal/ceramic interface to that in the bulk metal can then be expressed as $E_{\mathrm{f}}^{\mathrm{V}_{\mathrm{m}}^{\times}}(0)/E_{\mathrm{f}}^{\mathrm{V}_{\mathrm{m}}^{\times}}(\infty) = (N_b - N_s)/N_b + (N_s/N_b) W_{\mathrm{ad}}/\gamma_{\mathrm{m}}$.

Of course, a simplistic bond model is only heuristic; we therefore, only retain the basic functional form: $E_{\mathrm{f}}^{\mathrm{V}_{\mathrm{m}}^{\times}}(0)/E_{\mathrm{f}}^{\mathrm{V}_{\mathrm{m}}^{\times}}(\infty) = A + B\,(W_{\mathrm{ad}}/\gamma_{\mathrm{m}})$.

To find the two constants $A$ and $B$, we augmented our Ni/$Al_2O_3$ calculations with similar calculations for Cu/$Al_2O_3$ in the same orientation and obtained $W_{\mathrm{ad}}$ from experiment [24] and $\gamma_{\mathrm{m}}$ from DFT [25]. This yields $A = 0.03$ and $B = 1.09$. Given the accuracy of these calculations, we approximate this as $A = 0$ and $B = 1$; which yields the simple result presented as Eq. (1) in the manuscript:

$$\frac{E_{\mathrm{f}}^{\mathrm{V}_{\mathrm{m}}^{\times}}(0)}{E_{\mathrm{f}}^{\mathrm{V}_{\mathrm{m}}^{\times}}(\infty)} = \frac{W_{\mathrm{ad}}}{\gamma_{\mathrm{m}}}. \tag{24}$$

---


[1] L Klinger and E Rabkin. Theory of the kirkendall effect during grain boundary interdiffusion. *Acta Materialia*, 59(4):1389–1399, 2011.

[2] W Craig Carter, Andrew R Roosen, John W Cahn, and Jean E Taylor. Shape evolution by surface diffusion and surface attachment limited kinetics on completely faceted surfaces. *Acta metallurgica et materialia*, 43(12):4309–4323, 1995.

[3] L Klinger and E Rabkin. Effects of surface anisotropy on grain boundary grooving. *Interface science*, 9(1-2):55–63, 2001.

[4] Sergiy V Divinski, Gerrit Reglitz, and Gerhard Wilde. Grain boundary self-diffusion in polycrystalline nickel of different purity levels. *Acta Materialia*, 58(2):386–395, 2010.

[5] JM Blakely and H Mykura. Surface self diffusion measurements on nickel by the mass transfer method. *Acta Metallurgica*, 9(1):23–31, 1961.

[6] Hila Meltzman, Dominique Chatain, Dan Avizemer, Theodore M Besmann, and Wayne D Kaplan. The equilibrium crystal shape of nickel. *Acta Materialia*, 59(9):3473–3483, 2011.

[7] D. Prokoshkina, V.A. Esin, G. Wilde, and S.V. Divinski. Grain boundary width, energy and self-diffusion in nickel: effect of material purity. *Acta Materialia*, 61(14):5188–5197, 2013.

[8] Haowei Peng, Zeng-Hui Yang, John P Perdew, and Jianwei Sun. Versatile van der waals density functional based on a meta-generalized gradient approximation. *Physical Review X*, 6(4):041005, 2016.

[9] Charles Kittel. *Introduction to solid state physics*. Wiley, 2005.

[10] WR Tyson and WA Miller. Surface free energies of solid metals: Estimation from liquid surface tension measurements. *Surface Science*, 62(1):267–276, 1977.

[11] Alexey A Sokol, Aron Walsh, and C Richard A Catlow. Oxygen interstitial structures in close-packed metal oxides. *Chemical Physics Letters*, 492(1):44–48, 2010.

[12] Yu V Shvyd'ko, M Lucht, E Gerdau, M Lerche, EE Alp, W Sturhahn, J Sutter, and TS Toellner. Measuring wavelengths and lattice constants with the mössbauer wavelength standard. *Journal of Synchrotron Radiation*, 9(1):17–23, 2002.

[13] Katsuyuki Matsunaga, Tomohito Tanaka, Takahisa Yamamoto, and Yuichi Ikuhara. First-principles calculations of intrinsic defects in $Al_2O_3$. *Physical Review B*, 68(8):085110, 2003.

[14] David R Lide. CRC handbook of chemistry and physics: A ready-reference book of chemical and physical data, 2004.

[15] Donald J Siegel, Louis G Hector Jr, and James B Adams. Adhesion, atomic structure, and bonding at the Al (111)/$\alpha$-$Al_2O_3$ (0001) interface: A first principles study. *Physical Review B*, 65(8):085415, 2002.

[16] JM McHale, A Auroux, AJ Perrotta, and A Navrotsky. Surface energies and thermodynamic phase stability in nanocrystalline aluminas. *Science*, 277(5327):788–791, 1997.

[17] Roger H French. Electronic band structure of $Al_2O_3$, with comparison to AlON and AIN. *Journal of the American Ceramic Society*, 73(3):477–489, 1990.

[18] Christoph Freysoldt, Blazej Grabowski, Tilmann Hickel, Jörg Neugebauer, Georg Kresse, Anderson Janotti, and Chris G Van de Walle. First-principles calculations for point defects in solids. *Reviews of Modern Physics*, 86(1):253, 2014.

[19] G Makov and MC Payne. Periodic boundary conditions in ab initio calculations. *Physical Review B*, 51(7):4014, 1995.

[20] Donghwa Lee, Jonathan L DuBois, and Vincenzo Lordi. Identification of the local sources of paramagnetic noise in superconducting qubit devices fabricated on $\alpha$-$Al_2O_3$ substrates using density-functional calculations. *Physical Review Letters*, 112(1):017001, 2014.

[21] NDM Hine, K Frensch, WMC Foulkes, and MW Finnis. Supercell size scaling of density functional theory formation energies of charged defects. *Physical Review B*, 79(2):024112, 2009.

[22] Vitaly Alexandrov, Maria L. Sushko, Daniel K. Schreiber, Stephen M. Bruemmer, and Kevin M. Rosso. Ab initio modeling of bulk and intragranular diffusion in ni alloys. *The*

*Journal of Physical Chemistry Letters*, 6(9):1618–1623, 2015.

[23] MW Finnis and JE Sinclair. A simple empirical n-body potential for transition metals. *Philosophical Magazine A*, 50(1):45–55, 1984.

[24] D Chatain, I Rivollet, and N Eustathopoulos. Adhésion thermodynamique dans les systèmes non-réactifs métal liquide-alumine. *Journal de Chimie Physique*, 83:561–567, 1986.

[25] Richard Tran, Zihan Xu, Donald Winston Balachandran Radhakrishnan, Wenhao Sun, Kristin A Persson, and Shyue Ping Ong. Surface energies of elemental crystals. *Scientific Data*, 3, 2016.
